# Supplementary material for: Impulsively Excited Gravitational Quantum States: Echoes and Time-resolved Spectroscopy
Source: arXiv:2009.11755 ancillary file (2020-09-24)
Supplement: Supplementary file 1 [file sup_mat.pdf]

# Supplemental Material: "Impulsively Excited Gravitational Quantum States: Echoes and Time-resolved Spectroscopy"

I. Tutunnikov,[1] K. V. Rajitha,[1] A. Yu. Voronin,[2] V. V. Nesvizhevsky,[3] and I. Sh. Averbukh[1]

[1] *AMOS and Department of Chemical and Biological Physics, The Weizmann Institute of Science, Rehovot 7610001, Israel*

[2] *Lebedev Institute, 53 Leninsky pr., Moscow, Russia, Ru-119333*

[3] *Institut Max von Laue-Paul Langevin (ILL), 71 avenue des Martyrs, Grenoble, France, F-38042*

This Supplemental Material covers some technical details related to the results presented in the Letter. In Sec. A, matrix elements needed for describing the interaction with inhomogeneous magnetic field are provided. In Sec. B, our approach to solving the problem with the time-dependent boundary position is outlined. In Sec. C, we use the time-dependent perturbation theory (in the limit of weak kicks) to derive the expression for the ground state population as a function of the kick delay, $|c_1|^2(\tau)$.

### A. Kick by a pulsed inhomogeneous magnetic field

The time-dependent Schrödinger equation with the Hamiltonian $H = H_{\rm g} - s\beta(t)z$ [for definition of $H_{\rm g}$, see Eq. (1) in the Letter] is solved by expanding the QB's wave function $\Psi(z,t)$ in the basis of the eigenfunctions $\psi_m$s [see Eq. (2) in the Letter] of the Hamiltonian $H_{\rm g}$. The matrix elements of the interaction potential, $-s\beta(t)z$ in the basis of $\psi_m$s are evaluated using the integral (see [1, 2])

$$\int_0^\infty \psi_m^* z \psi_n\, dz = \begin{cases} (-1)^{n-m+1}\frac{2}{(z_m-z_n)^2}, & m \neq n \\ \frac{2}{3}z_m, & m = n \end{cases}. \quad (1)$$

### B. Kick by a jolt from the moving surface

In order to solve the problem with the time-dependent boundary condition $\Psi[z = h(t)] = 0$, it is advantageous to make a coordinate transformation into the rest frame of the surface, $w = z - h(t)$. Then, the motion of the QB is described by the time-dependent Shrödinger equation [in the units defined under Eq. (1) in the Letter]

$$\left(H_{\rm g} + i\dot{h}\partial_w\right)\Psi(w,t) = i\partial_t \Psi(w,t), \quad (2)$$

with time-independent boundary conditions, $\Psi(w = 0,t) = \Psi(w \to \infty, t) = 0$. The matrix elements of the interaction potential, $i\dot{h}\partial_w$ between the eigenfunctions $\psi_m$s are given by

$$i\dot{h}\int_0^\infty \psi_m^* \partial_w \psi_n\, dw = i\dot{h}\begin{cases} \frac{(-1)^{m+n}}{z_m-z_n}, & m \neq n \\ 0, & m = n \end{cases}. \quad (3)$$

Equation (3) is derived as follows. We consider real normalized eigenfunctions, $\psi_m(z) = N_m \mathrm{Ai}(z-z_m) = \mathrm{Ai}(z-z_m)|\mathrm{Ai}'(-z_m)|^{-1}$, and denote derivatives $\partial_x f(x-a)$ as $f'(x-a)$. We begin by considering the auxiliary integral $\int_0^\infty \left[\mathrm{Ai}'(z-z_m)\mathrm{Ai}'(z-z_n)\right]' dz$. On the one hand,

$$\int_0^\infty \left[\mathrm{Ai}'(z-z_m)\mathrm{Ai}'(z-z_n)\right]' dz = -\mathrm{Ai}'(-z_m)\mathrm{Ai}'(-z_n), \quad (4)$$

but on the other hand

$$\int_0^\infty \left[\mathrm{Ai}'(z-z_m)\mathrm{Ai}'(z-z_n)\right]' dz = \int_0^\infty \mathrm{Ai}''(z-z_m)\mathrm{Ai}'(z-z_n)\, dz + \int_0^\infty \mathrm{Ai}'(z-z_m)\mathrm{Ai}''(z-z_n)\, dz. \quad (5)$$

Using the property of the Airy function $\mathrm{A}''(z-z_m) = (z-z_m)\mathrm{A}(z-z_m)$ and integration by parts, Eq. (5) can be reduced to

$$\int_0^\infty \left[\mathrm{Ai}'(z-z_m)\mathrm{Ai}'(z-z_n)\right]' dz = = -(z_m - z_n)\int_0^\infty \mathrm{Ai}(z-z_m)\mathrm{Ai}'(z-z_n)\, dz. \quad (6)$$

Comparing Eq. (4) with Eq. (6) results in

$$\int_0^\infty \mathrm{Ai}(z-z_m)\mathrm{Ai}'(z-z_n)\, dz = = \begin{cases} \frac{\mathrm{Ai}'(-z_m)\mathrm{Ai}'(-z_n)}{z_m-z_n}, & m \neq n \\ 0, & m = n \end{cases}. \quad (7)$$

Finally, we substitute the normalization constants [see Eq. (2) in the Letter] and obtain

$$V_{mn} = \int_0^\infty \psi_m \psi_n'\, dw = \frac{1}{|\mathrm{Ai}'(-z_m)|}\frac{1}{|\mathrm{Ai}'(-z_n)|}\frac{\mathrm{Ai}'(-z_m)\mathrm{Ai}'(-z_n)}{z_m - z_n} = = \frac{(-1)^{m+n}}{z_m - z_n}. \quad (8)$$

### C. Population of the ground state as a function of the kick delay

We assume that the surface displacements are small, $a_{\rm k1}, a_{\rm k2} \ll 1$. In addition, to simplify the formulas (but

without loss of generality), we assume that both kicks are the same ($a_{\mathrm{k}1} = a_{\mathrm{k}2} = a_{\mathrm{k}}$, $\sigma_{\mathrm{k}1} = \sigma_{\mathrm{k}2} = \sigma_{\mathrm{k}}$), such that the surface height during each kick is given by $h(t) = a_{\mathrm{k}} \exp[-(t/\sigma_{\mathrm{k}})^2]$.

At the first order in perturbation theory, the ground state population, $|c_1|^2$ as a function of the delay between the kicks, $\tau$ is given by

$$|c_1|^2(\tau) = 1 - 2A^2 \sum_{m=2}^{\infty} e^{-\sigma_{\mathrm{k}}^2 f_{m1}^2/2} \cos(f_{m1}\tau), \qquad (9)$$

where $A = \sqrt{\pi} a_{\mathrm{k}} \sigma_{\mathrm{k}}$, and $f_{m1} = z_m - z_1$ [where $z_m$ are the energies of the GQSs, see Eq. (2) in the Letter]. The derivation of Eq. (9) is summarized below.

The time-dependent wave function of the QB is $\Psi(z,t) = \sum_{m=1}^{\infty} c_m e^{-iz_m t}\psi_m$. Assuming the initial state of the QB is the ground state, $c_m = \delta_{m1}$, where $\delta_{mn}$ is the Kronecker delta. In the first order of the perturbation theory, the expansion coefficients $c_m^{\mathrm{I}}$ just after the first kick are given by

$$\begin{aligned} c_m^{\mathrm{I}} &\approx \delta_{m1} + V_{m1} \int_{-\infty}^{\infty} \dot{h}(t) e^{i f_{m1} t}\, dt. \\ &= \delta_{m1} - i\sqrt{\pi} a_{\mathrm{k}} \sigma_{\mathrm{k}} V_{m1} f_{m1} e^{-\sigma_{\mathrm{k}}^2 f_{m1}^2/4} \\ &= \delta_{m1} - i\sqrt{\pi} a_{\mathrm{k}} \sigma_{\mathrm{k}} \frac{(-1)^{m+1}}{(z_m - z_1)} (z_m - z_1) e^{-\sigma_{\mathrm{k}}^2 f_{m1}^2/4} \\ &= \begin{cases} i(-1)^m A e^{-\sigma_{\mathrm{k}}^2 f_{m1}^2/4}, & m \neq 1 \\ 1, & m = 1 \end{cases}. \end{aligned} \qquad (10)$$

Here $V_{mn}$ is given by Eq. (8), $A = \sqrt{\pi} a_{\mathrm{k}} \sigma_{\mathrm{k}}$, and $f_{m1} = z_m - z_1$ [see Eq. (2) in the Letter]. After a delay $\tau$, the QB is kicked again. The expansion coefficient of the ground state after the second kick is given by

$$\begin{aligned} c_1^{\mathrm{II}} &= c_1^{\mathrm{I}} e^{-iz_1\tau} + \sum_{m=1}^{\infty} V_{1m} c_m^{\mathrm{I}} e^{-iz_m\tau} \\ &\times \int_{-\infty}^{\infty} \dot{h}(t-\tau) e^{i f_{1m} t}\, dt = \end{aligned} \qquad (11)$$

$$\begin{aligned} &= e^{-iz_1\tau} - i\sqrt{\pi} a_{\mathrm{k}} \sigma_{\mathrm{k}} \sum_{m=1}^{\infty} V_{1m} c_m^{\mathrm{I}} e^{-iz_m\tau} f_{1m} e^{-\sigma_{\mathrm{k}}^2 f_{1m}^2/4} \\ &= e^{-iz_1\tau} + i\sqrt{\pi} a_{\mathrm{k}} \sigma_{\mathrm{k}} \sum_{m=2}^{\infty} (-1)^m c_m^{\mathrm{I}} e^{-iz_m\tau} e^{-\sigma_{\mathrm{k}}^2 f_{1m}^2/4} \\ &= e^{-iz_1\tau} - A^2 \sum_{m=2}^{\infty} e^{-\sigma_{\mathrm{k}}^2 f_{m1}^2/2} e^{-iz_m\tau}. \end{aligned} \qquad (12)$$

Finally, the population of the ground state after the second kick takes the form of Eq. (9). In agreement with Eq. (4) in the Letter, the signal contains the transition frequencies between the excited states $\psi_m$ and the ground state $\psi_1$.


[1] J. R. Albright, *"Integrals of products of Airy functions,"* J. Phys. A **10**, 485 (1977).

[2] J. Gea-Banacloche, *"A quantum bouncing ball,"* Am. J. Phys **67**, 776 (1999).
